# Supplementary material for: Highly comparative feature-based time-series classification
Source: arXiv:1401.3531 source file (2014-05-09)
Supplement: Supplementary file 1 [file datamining_supplement.pdf]

# Supplementary Material: Highly comparative, feature-based time-series classification

Ben D. Fulcher and Nick S. Jones

In this document we provide additional information to accompany the findings presented in *Highly comparative feature-based time-series classification*.

### *UCR Datasets*

In Table I, we provide a table with details of all twenty UCR time-series datasets analyzed in this work, including the number of classes, $n_{\mathrm{classes}}$, the number of training examples, $n_{\mathrm{train}}$, the number of test examples, $n_{\mathrm{test}}$, and the number of samples making up each time series in the dataset, $N$.

### *Low-dimensional representation of the Swedish Leaf dataset*

In previous work we reported that useful representations of time-series datasets can be obtained by projecting them onto low-dimensional feature spaces using dimensionality reduction methods like principal components analysis [19]. Here we use the example of the Swedish Leaf dataset to show that similarly informative projections can also be formed for some of the datasets studied here, even though their class labels are not used. We normalized features (as per [19]) and used principal components analysis to produce the two-dimensional feature-based representation of the dataset shown in Suppl. Fig. 1A. The dendrogram shown in Suppl. Fig. 1B reflects a linkage clustering of the distances between cluster centers in this two-dimensional space.

B. D. Fulcher is with the Department of Physics, University of Oxford, UK. Email: ben.d.fulcher@gmail.com

N. S. Jones is with the Department of Mathematics, Imperial College London, UK. Email: nick.jones@imperial.ac.uk

TABLE I

**The twenty time-series datasets analyzed in this work, as obtained from 'The UCR Time Series Classification/Clustering Homepage' [1].** For each dataset, we list the number of classes, $n_{\mathrm{classes}}$, the number of training examples, $n_{\mathrm{train}}$, the number of test examples, $n_{\mathrm{test}}$, and the length of each time series, $N$. References are given to the first published work to use each dataset.

| Dataset | $n_{\mathrm{classes}}$ | $n_{\mathrm{train}}$ | $n_{\mathrm{test}}$ | $N$ (samples) |
|---|---|---|---|---|
| *Synthetic Control* [2] | 6 | 300 | 300 | 60 |
| *Gun point* [3] | 2 | 50 | 150 | 150 |
| *CBF* [4] | 3 | 30 | 900 | 128 |
| *Face (all)* [5] | 14 | 560 | 1690 | 131 |
| *OSU Leaf* [6] | 6 | 200 | 242 | 427 |
| *Swedish Leaf* [7] | 15 | 500 | 625 | 128 |
| *50 Words* [8] | 50 | 450 | 455 | 270 |
| *Trace* [9] | 4 | 100 | 100 | 275 |
| *Two Patterns* [10] | 4 | 1 000 | 4 000 | 128 |
| *Wafer* [11] | 2 | 1 000 | 6 164 | 152 |
| *Face (four)* [5] | 4 | 24 | 88 | 350 |
| *Lightning (two)* [12] | 2 | 60 | 61 | 637 |
| *Lightning (seven)* [12] | 7 | 70 | 73 | 319 |
| *ECG* [11] | 2 | 100 | 100 | 96 |
| *Adiac* [13] | 37 | 390 | 391 | 176 |
| *Yoga* [14] | 2 | 300 | 3 000 | 426 |
| *Fish* [15] | 7 | 175 | 175 | 463 |
| *Beef* [16] | 5 | 30 | 30 | 470 |
| *Coffee* [17] | 2 | 28 | 28 | 286 |
| *Olive Oil* [18] | 4 | 30 | 30 | 570 |

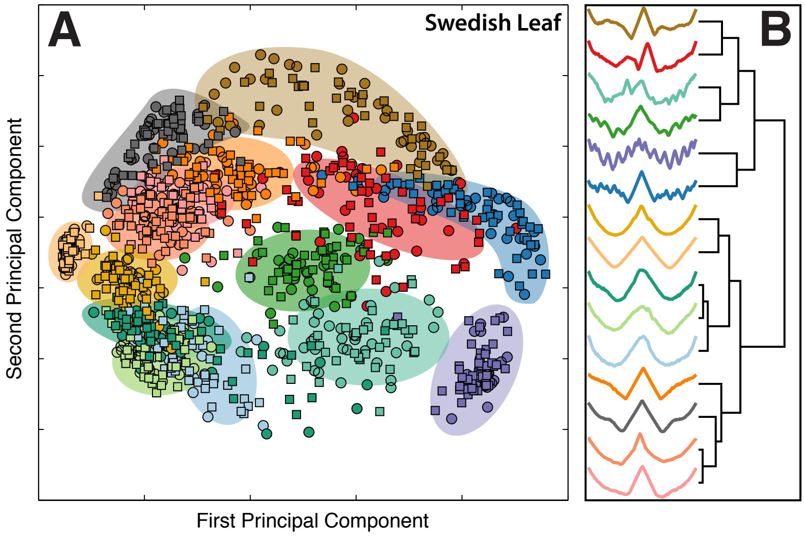


Supplementary Figure 1. **A feature-based principal components projection of the Swedish Leaf dataset. A** The training (circles) and test (squares) data of the Swedish Leaf dataset are plotted in the space of the first two principal components of the normalized feature space for this dataset. Note that this is an unsupervised representation of the dataset and neither the training and testing labels, nor the class assignments were used to construct the low-dimensional representation. Nevertheless, different labeled classes of leaf patterns occupy characteristic regions of the space and similar leaf patterns are placed near one another. **B** A dendrogram constructed between class centers in this space using average linkage clustering reflects a visually intuitive structuring of the types of leaf patterns in this dataset.

*Two Patterns dataset*

In addition to the example shown for the Synthetic Control dataset in the main text, the Two Patterns dataset [10] provides an additional example of the interpretability of features selected using our highly comparative method. The four classes of time series that make up this dataset are illustrated in Suppl. Fig. 2B, and the two features selected by greedy forward feature selection are used to represent the full dataset in Suppl. Fig. 2A. The first feature is the time-averaged third-order quantity, $\langle (x_{t+\tau} - x_t)^3 \rangle$, where $\tau$ is chosen as the first minimum of the autocorrelation function, and the average $\langle \cdot \rangle$ is performed across the time series. This feature effectively distinguishes classes 1 (green) and 4 (pink), but confuses classes 2 (orange) and 3 (blue). The second selected feature, **SY_SpreadRandomLocal_100_meanmean**, computes the mean in one hundred randomly-selected 100-sample segments from the $z$-scored time series and returns the mean of this set of local means[1], and is complementary: compensating for the shortcoming of the first feature by effectively distinguishing classes 2 (orange) and 3 (blue). A linear classifier using these two features yields a test-set misclassification rate of 7.4%. Although 1-NN instance-based classification using DTW can achieve perfect classification for this dataset, this example demonstrates how a simple linear classifier using two extracted features provides an intuitive space in which to represent the dataset, with visually-interpretable results.

*Partition dependence*

The dependence of test set misclassification rates on training/test partitions for a 1-NN Euclidean classifier and our linear feature-based classifier are shown in Table II. In most cases the fixed partition provides a representative classification rate across repartitions, but in others the fixed partition provides an optimistic result (linear feature-based classifier for *Olive Oil*) or a pessimistic result (1-NN Euclidean for *Face (all)*) compared to what might be expected from a random assignment of training and testing labels. The variation in misclassification rates across different training/test partitions, as seen from the standard deviation across partitions, varies relatively widely across the datasets, and between the two classification methods, and can be an important quantity for judging the performance of a classifier on a given dataset, rather than simply optimizing performance for a given fixed data partition.

[1]For this dataset, time series are 128 samples long, so the set of local 100-sample means are contiguous 78% segments of the time series, that include the middle portion of each time series. Since time series in class 2 (plotted orange in Suppl. Fig. 2A) have 'dip, peak, peak, dip' patterns, and those in class 3 (plotted blue in Suppl. Fig. 2A) have the pattern 'peak, dip, dip, peak', segments of the time series that include this middle portion will be high for class 2 and low for class 3, contributing to their separation using this feature.

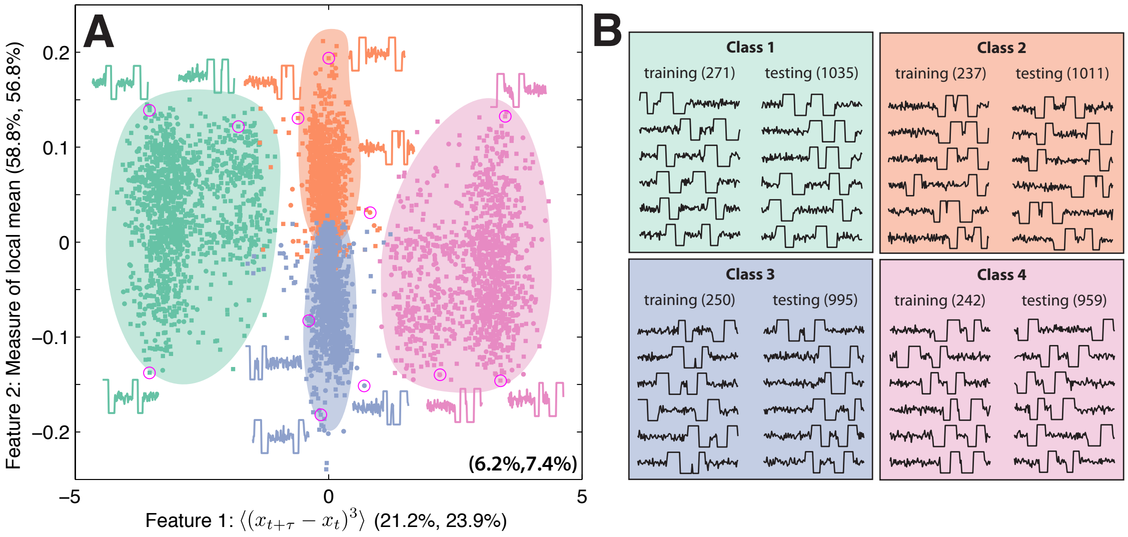


Supplementary Figure 2. **Highly comparative feature-based classification of the Two Patterns dataset. A** The Two Patterns dataset is plotted in the space of the two features selected to classify it. Linear discriminant misclassification rates are shown as percentages in the form (training, test) in the label for each individual feature, and for their combination, which is annotated in the bottom righthand corner of the plot. The 1 000 time series in the training set are plotted as circles, and the 4 000 time series in the test set are plotted as squares. Selected time series are annotated to the plot, as indicated by pink circles, and background shading has been added manually to guide the eye to each of the four classes, labeled as green, orange, blue, and pink. **B** The four classes are visualized by plotting 6 random time series in both the training and test sets.

TABLE II

**COMPARISON OF TEST SET MISCLASSIFICATION RATES FOR 1-NN EUCLIDEAN AND OUR LINEAR FEATURE-BASED CLASSIFIER OVER 50 REPARTITIONS OF THE TRAINING AND TEST DATA COMPARED TO THE FIXED TRAINING/TEST PARTITION PROVIDED FROM THE DATA SOURCE [1].** REPARTITIONS REPRESENT RANDOM ASSIGNMENTS OF THE TIME SERIES BETWEEN TRAINING AND TEST SETS, WHILE MAINTAINING THE CLASS PROPORTIONS OF THE FIXED PARTITION PROVIDED FROM THE DATA SOURCE. THE RESULTS FROM 50 REPARTITIONS ARE SUMMARIZED AS MEAN ± STANDARD DEVIATION.

| **Dataset** | **1-NN Euclidean** | | **Linear feature-based classifier** | | | |
|---|---|---|---|---|---|---|
| | Test set misclassification rate (%) | | Number of features | | Test set misclassification rate (%) | |
| | Fixed partition | 50 repartitions | Fixed partition | 50 repartitions | Fixed partition | 50 repartitions |
| *Synthetic Control* [2] | 12.0 | 10.1 ± 1.2 | 2 | 2.0 ± 0.0 | 3.7 | 2.5 ± 0.7 |
| *Gun point* [3] | 8.7 | 11.0 ± 2.9 | 2 | 1.2 ± 0.4 | 7.3 | 8.9 ± 2.9 |
| *CBF* [4] | 14.8 | 13.3 ± 4.2 | 2 | 1.7 ± 0.5 | 28.9 | 11.7 ± 7.7 |
| *Face (all)* [5] | 28.6 | 12.3 ± 2.6 | 5 | 5.9 ± 1.3 | 29.2 | 29.4 ± 8.1 |
| *OSU Leaf* [6] | 48.3 | 41.8 ± 2.4 | 5 | 4.4 ± 0.6 | 16.5 | 17.9 ± 4.2 |
| *Swedish Leaf* [7] | 21.1 | 22.8 ± 1.3 | 5 | 5.0 ± 0.8 | 22.7 | 15.8 ± 3.9 |
| *50 Words* [8] | 36.9 | 34.4 ± 1.4 | 7 | 6.7 ± 1.7 | 45.3 | 50.6 ± 9.4 |
| *Trace* [9] | 24.0 | 22.2 ± 3.9 | 1 | 1.0 ± 0.0 | 1.0 | 0.6 ± 1.0 |
| *Two Patterns* [10] | 9.3 | 9.6 ± 0.7 | 2 | 2.5 ± 0.6 | 7.4 | 5.8 ± 1.8 |
| *Wafer* [11] | 0.5 | 0.5 ± 0.1 | 1 | 1.0 ± 0.0 | 0.0 | 0.0 ± 0.0 |
| *Face (four)* [5] | 21.6 | 22.0 ± 5.5 | 3 | 2.3 ± 0.5 | 26.1 | 33.0 ± 8.7 |
| *Lightning (two)* [12] | 24.6 | 27.0 ± 4.9 | 2 | 2.8 ± 0.7 | 19.7 | 30.3 ± 7.5 |
| *Lightning (seven)* [12] | 42.5 | 39.7 ± 5.5 | 4 | 5.0 ± 0.9 | 43.8 | 40.3 ± 8.3 |
| *ECG* [11] | 12.0 | 12.1 ± 3.3 | 1 | 1.0 ± 0.0 | 1.0 | 1.7 ± 1.6 |
| *Adiac* [13] | 38.9 | 37.9 ± 1.8 | 5 | 4.9 ± 0.7 | 35.5 | 32.7 ± 3.2 |
| *Yoga* [14] | 17.0 | 16.0 ± 1.0 | 3 | 2.3 ± 0.7 | 22.6 | 25.9 ± 2.0 |
| *Fish* [15] | 21.7 | 19.9 ± 2.9 | 6 | 5.5 ± 1.0 | 17.1 | 22.4 ± 6.0 |
| *Beef* [16] | 46.7 | 53.5 ± 7.0 | 5 | 4.6 ± 1.4 | 43.3 | 47.6 ± 9.6 |
| *Coffee* [17] | 25.0 | 18.4 ± 7.8 | 1 | 1.0 ± 0.0 | 0.0 | 7.3 ± 6.0 |
| *Olive Oil* [18] | 13.3 | 14.3 ± 4.5 | 2 | 2.5 ± 0.5 | 10.0 | 24.8 ± 8.9 |

*Threshold dependence*

The number of features in our classifier is chosen as the point at which the improvement in training set classification accuracy from the addition of another feature drops below 3%. The dependence of our results on this choice is shown in Suppl. Fig. 3, for both mean test set misclassification rates (Suppl. Fig. 3A) and mean number of features selected (Suppl. Fig. 3B), where means are taken across all twenty datasets. At high thresholds, feature selection terminates earlier, producing classifiers with fewer features, whereas at low thresholds, feature selection continues further, producing classifiers containing a larger number of features, as shown in Suppl. Fig. 3B. The mean misclassification rate increases with the threshold, corresponding to better performance for classifiers containing more features, indicating that overfitting is not a large problem using our method with linear classifiers. Although differences in performance with the choice of threshold across this range of thresholds are not dramatic, the result indicates a level of trade-off between the extent of dimensionality reduction, i.e., the number of features in the resulting classifier, and its classification accuracy. The classification performance reported here is thus not very sensitive to our choice of 3%, with similar or better classification accuracies found for lower thresholds, for example. Note also that the trends shown in Suppl. Fig. 3 are not particular to linear classifiers, but were also seen for other types of classifiers (not shown).

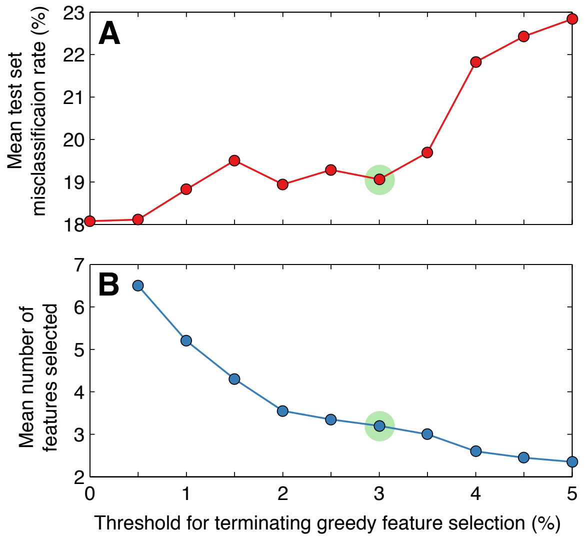


Supplementary Figure 3. **Dependence of test set misclassification rate and number of features selected, as a function of the threshold for terminating greedy forward feature selection.** Feature selection terminates when the improvement in training set classification rate from including an additional feature drops below this threshold. For the range of thresholds shown, the test set misclassification rate broadly increases with the size of the threshold whereas the number of features decreases. We use a threshold of 3% in this work (marked with a circle in both plots), although classification performance is not dramatically different across this range of thresholds.

*A List of Features Selected for Each Dataset*

Here we list the features selected for each dataset in turn, and note that code to evaluate each feature can be obtained by searching www.comp-engine.org/timeseries.

TABLE III: **Features selected for each dataset using greedy forward feature selection.** We provide the Matlab code for evaluating each function (where the input, x, is the time series, or y is the $z$-scored time series), although note that in general each code file will produce many outputs in a structure; the selected feature will be just a specific elements. A description of each feature, including Matlab code for evaluating it, is available at **www.comp-engine.org/timeseries**.

| Dataset | Selected feature name(s) | Matlab code |
|---|---|---|
| *Synthetic Control* | PH_ForcePotential_sine_10_004_10_median | PH_ForcePotential(y,‘sine’,[10,0.04,10]) |
| | SP_basic_pgram_hamm_power_q90mel | SP_Summaries(y,‘periodogram’,‘hamming’,[],0,1) |
| *Gun point* | SY_LocalDistributions_2_par_mindiv | SY_LocalDistributions(y,2,‘par’) |
| | CO_HistogramAMI_1_even_20 | CO_HistogramAMI(y,1,‘even’,20) |
| *CBF* | MF_armax_1_1_05_1_meanabs | MF_armax(y,[1,1],0.5,1) |
| | benmotif_bin_diff_uuuu | SB_MotifTwo(y,‘diff’) |
| *Face (all)* | CO_Embed2_tau_eucdm3 | CO_Embed2(y,‘tau’) |
| | DN_OutlierInclude_abs_mrm | DN_OutlierInclude(y,‘abs’) |
| | SP_basic_pgram_hamm_q50mel | SP_Summaries(y,‘periodogram’,‘hamming’,[],0,0) |
| | CO_trev_2_num | CO_trev(y,2) |
| | SP_basic_fft_power_fpolysat_rmse | SP_Summaries(y,‘fft’,[],[],0,1) |
| *OSU Leaf* | EN_SampEn_4_005_sampen4 | EN_SampEn(y,4,0.05) |
| | CO_HistogramAMI_4_std1_4 | CO_HistogramAMI(y,4,’std1’,4) |
| | MF_armax_2_2_05_1_MA_1 | MF_armax(y,[2,2],0.5,1) |
| | benmotif_tri_diffquant_ba | SB_MotifThree(y,‘diffquant’) |
| | EN_wentropy_threshent05 | EN_wentropy(y,‘threshold’,0.5) |
| *Swedish Leaf* | FC_LocalSimple_median7_meanabserr | FC_LocalSimple(y,‘median’,7) |
| | MF_armax_2_2_05_1_AR_1 | MF_armax(y,[2,2],0.5,1) |
| | PP_Compare_medianf10_kscn_relent | PP_Compare(x,‘medianf10’) |
| | MF_armax_2_2_05_1_maxdc | MF_armax(y,[2,2],0.5,1) |
| | SP_basic_pgram_hamm_area_5_3 | SP_Summaries(y,’periodogram’,’hamming’,[],0,1) |
| *50 Words* | MF_steps_ahead_ar_2_6_rmserr_2 | MF_steps_ahead(y,‘ar’,2,6) |
| | DN_OutlierInclude_abs_mrm | DN_OutlierInclude(y,‘abs’) |
| | DN_OutlierInclude_abs_nfla | DN_OutlierInclude(y,’abs’) |
| | NW_VisibilityGraph_horiz_evparm2 | NW_VisibilityGraph(y,‘horiz’) |
| | FC_Surprise_dist_20_2_q_mean | FC_Surprise(y,‘dist’,20,2,‘quantile’) |
| | benmotif_bin_diff_uuuu | SB_MotifTwo(y,‘diff’) |
| | MF_arfit_1_8_sbc_sbc_5 | MF_arfit(y,1,8,‘sbc’) |
| *Trace* | CO_trev_3_raw | CO_trev(y,3) |
| *Two Patterns* | CO_trev_ac_num | CO_trev(y,‘ac’) |

TABLE III: **(continued): Features selected for each dataset using greedy forward feature selection.**

| Dataset | Selected feature name(s) | Matlab code |
|---|---|---|
| | SY_SpreadRandomLocal_100_meanmean | SY_SpreadRandomLocal(y,100) |
| *Wafer* | benmotif_bin_diff_dudu | SB_MotifTwo(y,'diff') |
| *Face (four)* | SY_LocalDistributions_3_each_mindiv | SY_LocalDistributions(y,3,'each') |
| | PP_Compare_rav4_kscn_relent | PP_Compare(x,'rav4') |
| | DN_OutlierInclude_abs_nflb | DN_OutlierInclude(y,'abs') |
| *Lightning (two)* | CP_l1pwc_sweep_lambda_0_005_095_rmserrsu02 | CP_l1pwc_sweep_lambda(y,0:0.05:0.95) |
| | SP_basic_fft_power_fpolysat_a | SP_Summaries(y,'fft',[],[],0,1) |
| *Lightning (seven)* | CO_Embed2_tau_mean_eucds | CO_Embed2(y,'tau') |
| | SY_SlidingWindow_ent_s5_10 | SY_SlidingWindow(y,'ent','std',5,10) |
| | CO_TSTL_amutual_20_ami8 | CO_TSTL_amutual(y,20,[]) |
| | SP_basic_pgram_hamm_mom7 | SP_Summaries(y,'periodogram','hamming',[],0,0) |
| *ECG* | standard_deviation | DN_Spread(x,'std') |
| *Adiac* | CO_glscf_1_1_1 | CO_glscf(y,1,1,1) |
| | DN_RemovePoints_min_01_skewnessrat | DN_RemovePoints(y,'min',0.1) |
| | DN_SimpleFit_gauss2_r2_ks | DN_SimpleFit(y,'gauss2',0) |
| | FC_LocalSimple_median3_ac1 | FC_LocalSimple(y,'median',3) |
| | DN_RemovePoints_min_05_ac3rat | DN_RemovePoints(y,'min',0.5) |
| *Yoga* | MF_armax_1_1_05_1_maxdc | MF_armax(y,[1,1],0.5,1) |
| | FC_LocalSimple_meantau_meanabserr | FC_LocalSimple(y,'mean','ac') |
| | PP_Compare_resample_2_1_statav6 | PP_Compare(x,'resample_2_1') |
| *Fish* | EX_MovingThreshold_01_002_iqrq | EX_MovingThreshold(y,0.1,0.02) |
| | PH_Walker_biasprop_01_05_w_mean | PH_Walker(y,'biasprop',[0.1,0.5]) |
| | SC_FluctAnal_2_dfa_25_1_2_logi_ratsplitminerr | SC_FluctAnal(y,2,'dfa',25,1,2,1) |
| | CP_ML_StepDetect_l1pwc_005_rmsoff | CP_ML_StepDetect(y,'l1pwc',0.05) |
| | TSTL_localdensity_5_40_ac_2_stdden | TSTL_localdensity(y,5,40,'ac',2) |
| | MF_steps_ahead_arma_3_1_6_mabserr_1 | MF_steps_ahead(y,'arma',[3,1],6) |
| *Beef* | SP_basic_pgram_hamm_fpoly2csS_p2 | SP_Summaries(y,'periodogram','hamming',[],0,1) |
| | SC_FluctAnal_2_iqr_1_ratsplitminerr | SC_FluctAnal(y,2,'iqr',1,[],[],0) |
| | SP_basic_pgram_hamm_cep_area_4_4 | SP_Summaries(y,'periodogram','hamming',[],1,0) |
| | benmotif_bin_diff_ddu | SB_MotifTwo(y,'diff') |
| | PP_Iterate_resampleup_gauss1_h10_lin | PP_Iterate(x,'resampleup') |
| *Coffee* | CO_trev_2_absnum | CO_trev(y,2) |
| *Olive Oil* | PP_Iterate_spline_swms5_2_exp | PP_Iterate(x,'spline') |
| | DN_RemovePoints_max_01_median | DN_RemovePoints(y,'max',0.1) |

## REFERENCES


[1] E. Keogh, X. Xi, L. Wei, and C. A. Ratanamahatana. (2006) The UCR Time Series Classification/Clustering Homepage. [Online]. Available: www.cs.ucr.edu/~eamonn/time_series_data/

[2] D. T. Pham and A. B. Chan, "Control chart pattern recognition using a new type of self-organizing neural network," *Proc. Inst. Mech. Eng. I-J. Sys.*, vol. 212, no. 2, pp. 115–127, 1998.

[3] C. A. Ratanamahatana and E. Keogh, "Making time-series classification more accurate using learned constraints," in *SIAM Int'l Conf. Data Mining*, 2004.

[4] N. Saito, "Local feature extraction and its applications using a library of bases," Ph.D. dissertation, Yale University, 1994.

[5] C. A. Ratanamahatana and E. Keogh, "Everything you know about Dynamic Time Warping is wrong," in *Third Workshop on Mining Temporal and Sequential Data, in conjunction with the Tenth ACM SIGKDD International Conference on Knowledge Discovery and Data Mining*, Seattle, WA, USA, 2004, pp. 22–25.

[6] A. Gandhi, "Content-based image retrieval: Plant species identification," *Master's thesis, Oregon State University*, 2002.

[7] O. J. O. Söderkvist, "Computer vision classification of leaves from Swedish trees," Master's thesis, 2001.

[8] T. Rath and R. Manmatha, "Word image matching using Dynamic Time Warping," in *IEEE Conference on Computer Vision and Pattern Recognition*, vol. 2. IEEE Computer Society, 2003, p. 521.

[9] D. Roverso, "Multivariate temporal classification by windowed wavelet decomposition and recurrent neural networks," in *3rd ANS Int'l Topical Meeting on Nuclear Plant Instrumentation, Control and Human-Machine Interface*, vol. 20, Washington, DC, USA, 2000.

[10] P. Geurts, "Contributions to decision tree induction: bias/variance tradeoff and time series classification," Ph.D. dissertation, Department of Electrical Engineering, University of Liege, Belgium, 2002.

[11] R. T. Olszweski, "Generalized feature extraction for structural pattern recognition in time-series data," Ph.D. dissertation, Carnegie Mellon University, Pittsburgh, PA, USA, 2001.

[12] D. Eads, D. Hill, S. Davis, S. Perkins, J. Ma, R. Porter, and J. Theiler, "Genetic algorithms and support vector machines for time series classification," in *Applications and Science of Neural Networks, Fuzzy Systems, and Evolutionary Computation V*, B. Bosacchi, D. B. Fogel, and J. C. Bezdek, Eds., vol. 4787, Seattle, WA, USA, 2002, pp. 74–85.

[13] A. Jalba, M. Wilkinson, J. Roerdink, M. Bayer, and S. Juggins, "Automatic diatom identification using contour analysis by morphological curvature scale spaces," *Mach. Vision Appl.*, vol. 16, pp. 217–228, 2005. [Online]. Available: http://dx.doi.org/10.1007/s00138-005-0175-8

[14] L. Wei and E. Keogh, "Semi-supervised time series classification," in *Proc. of the 12th ACM SIGKDD Int'l Conf. Knowledge Discovery and Data Mining*, vol. 20, no. 23, New York, NY, USA, 2006, pp. 748–753.

[15] D.-J. Lee, R. B. Schoenberger, D. Shiozawa, X. Xu, and P. Zhan, "Contour matching for a fish recognition and migration-monitoring system," in *Proc. SPIE, Two- and Three-Dimensional Vision Systems for Inspection,*

*Control, and Metrology II*, vol. 5606, no. 1. Philadelphia, PA, USA: International Society for Optics and Photonics, 2004, pp. 37–48. [Online]. Available: http://dx.doi.org/doi/10.1117/12.571789

[16] O. Al-Jowder, E. K. Kemsley, and R. H. Wilson, "Detection of adulteration in cooked meat products by mid-infrared spectroscopy," *J. Agr. Food Chem.*, vol. 50, no. 6, pp. 1325–1329, 2002. [Online]. Available: http://pubs.acs.org/doi/abs/10.1021/jf0108967

[17] R. Briandet, E. K. Kemsley, and R. H. Wilson, "Discrimination of Arabica and Robusta in instant coffee by Fourier transform infrared spectroscopy and chemometrics," *J. Agr. Food Chem.*, vol. 44, no. 1, pp. 170–174, 1996. [Online]. Available: http://pubs.acs.org/doi/abs/10.1021/jf950305a

[18] H. S. Tapp, M. Defernez, and E. K. Kemsley, "FTIR spectroscopy and multivariate analysis can distinguish the geographic origin of extra virgin olive oils," *J. Agr. Food Chem.*, vol. 51, no. 21, pp. 6110–6115, 2003. [Online]. Available: http://pubs.acs.org/doi/abs/10.1021/jf030232s

[19] B. D. Fulcher, M. A. Little, and N. S. Jones, "Highly comparative time-series analysis: the empirical structure of time series and their methods," *J. Roy. Soc. Interface*, vol. 10, no. 83, p. 20130048, 2013.
